# Supplementary material for: Optimal finite-range atomic basis sets for liquid water and ice
Source: arXiv:1307.3187 source file (2013-11-11)
Supplement: Supplementary file 1 [file supplementary_material.pdf]

```
# arXiv:1307.3187 [physics.chem-ph]
#
# Supplementary Material for:
# Optimal finite-range atomic basis sets for liquid water and ice
# Fabiano Corsetti, M-V Fernández-Serra, José M Soler, Emilio Artacho
#
# Basis sets are given in SIESTA's fdf input format:
#
# %block PAO.Basis
# (name of atom) (number of shells for atom) (optional: additional charge given to atom)
# n=(principal quantum number) (orbital angular momentum) (zeta level) E (V_0) (r_i) Q (Q_0) (lambda)
#     (r_c) (r_dz) (r_tz) (r_qz) ...
# ...
# ...
# %endblock PAO.Basis
#
# The two parameters after E define the soft confinement, and the two after Q the Coulomb confinement
# Units:
#    V_0 : Rydberg Bohr
#    Q_0 : Rydberg Bohr
#    lambda : Bohr^-1
#    r_c, r_i, r_dz, r_tz, r_qz : Bohr
#
# Specifications for the (P)dz+p and (P)tz+p basis sets can be found in the Supplementary Material for:
# Wang J, Román-Pérez G, Soler J M, Artacho E and Fernández-Serra M V 2011 J. Chem. Phys. 134 024516

%block PAO.Basis # dz+p
O 3
n=2 0 2 E 50.0 7.5
     8.0 2.7
n=2 1 2 E 10.0 8.3
     8.5 2.6
n=3 2 1 E 40.0 8.3 Q  6.8 0.22
     8.5
H 2
n=1 0 2 E 50.0 8.3
     8.5 2.2
n=2 1 1 E 20.0 7.8 Q  6.5 0.90
     8.0
%endblock PAO.Basis

%block PAO.Basis # tz+p
O 3
n=2 0 3 E 50.0 7.5
     8.0 3.5 2.0
n=2 1 3 E 10.0 8.3
     8.5 3.4 2.0
n=3 2 1 E 40.0 8.3 Q  6.8 0.22
     8.5
H 2
n=1 0 3 E 50.0 8.3
     8.5 3.8 2.0
n=2 1 1 E 20.0 7.8 Q  6.5 0.90
     8.0
%endblock PAO.Basis

%block PAO.Basis # tz+d(H)p
O 3
n=2 0 3 E 50.0 7.5
     8.0 3.5 2.0
n=2 1 3 E 10.0 8.3
     8.5 3.4 2.0
n=3 2 1 E 40.0 8.3 Q  6.8 0.22
     8.5
H 2
n=1 0 3 E 50.0 8.3
     8.5 3.8 2.0
n=2 1 2 E 20.0 7.8 Q  3.5 0.00
     8.0 2.0
%endblock PAO.Basis
```

```
%block PAO.Basis # tz+dp
O 3
n=2 0 3 E 50.0 7.5
     8.0 3.5 2.0
n=2 1 3 E 10.0 8.3
     8.5 3.4 2.0
n=3 2 2 E 40.0 8.3 Q  6.0 0.00
     8.5 2.2
H 2
n=1 0 3 E 50.0 8.3
     8.5 3.8 2.0
n=2 1 2 E 20.0 7.8 Q  3.5 0.00
     8.0 2.0
%endblock PAO.Basis

%block PAO.Basis # tz+dp+p'
O 4
n=2 0 3 E 50.0 7.5
     8.0 3.5 2.0
n=2 1 3 E 10.0 8.3
     8.5 3.4 2.0
n=3 2 2 E 40.0 8.3 Q  6.0 0.00
     8.5 2.2
n=4 3 1 E 50.0 8.3 Q 17.0 0.40
     8.5
H 3
n=1 0 3 E 50.0 8.3
     8.5 3.8 2.0
n=2 1 2 E 20.0 7.8 Q  3.5 0.00
     8.0 2.0
n=3 2 1 E 50.0 8.3 Q 16.0 0.80
     8.5
%endblock PAO.Basis

%block PAO.Basis # (s)qz+dp
O 3
n=2 0 4 E 50.0 7.5
    8.0 5.0 3.5 2.0
n=2 1 4 E 10.0 8.3
    8.5 5.0 3.5 2.0
n=3 2 2 E 40.0 8.3 Q  6.0 0.00
    8.5 2.2
H 2
n=1 0 4 E 50.0 8.3
    8.5 5.0 3.5 2.0
n=2 1 2 E 20.0 7.8 Q  3.5 0.00
    8.0 2.0
%endblock PAO.Basis

%block PAO.Basis # qz+dp
O 3
n=2 0 4 E 50.0 8.0
   10.0 5.0 3.5 2.0
n=2 1 4 E 10.0 8.0
   10.0 5.0 3.5 2.0
n=3 2 2 E 40.0 9.0 Q  6.0 0.01
   10.0 2.2
H 2
n=1 0 4 E 50.0 8.0
   10.0 5.0 3.5 2.0
n=2 1 2 E 50.0 9.0 Q  3.5 0.01
   10.0 2.0
%endblock PAO.Basis
```

```
%block PAO.Basis # qz+dp+p'
O 4
n=2 0 4 E 50.0 8.0
   10.0 5.0 3.5 2.0
n=2 1 4 E 10.0 8.0
   10.0 5.0 3.5 2.0
n=3 2 2 E 40.0 9.0 Q  6.0 0.00
   10.0 2.2
n=4 3 1 E 50.0 9.0 Q 17.0 0.40
   10.0
H 3
n=1 0 4 E 50.0 9.0
   10.0 5.0 3.5 2.0
n=2 1 2 E 50.0 9.0 Q  3.5 0.00
   10.0 2.0
n=3 2 1 E 50.0 9.0 Q 16.0 0.80
   10.0
%endblock PAO.Basis

%block PAO.Basis # qz+dp+p'+s(O)d
O 4
n=2 0 4 E 50.0 8.0
   10.0 5.0 3.5 2.0
n=2 1 4 E 10.0 8.0
   10.0 5.0 3.5 2.0
n=3 2 2 E 40.0 9.0 Q  6.0 0.00
   10.0 2.2
n=4 3 1 E 50.0 9.0 Q 17.0 0.40
   10.0
O_ghost 2 -0.3 # ghost atom positioned on top of O with the same pseudopotential
n=2 0 1 E 50.0 8.0
   10.0
n=2 1 1 E 10.0 8.0
   10.0
H 3
n=1 0 4 E 50.0 9.0
   10.0 5.0 3.5 2.0
n=2 1 2 E 50.0 9.0 Q  3.5 0.00
   10.0 2.0
n=3 2 1 E 50.0 9.0 Q 16.0 0.80
   10.0
%endblock PAO.Basis

%block PAO.Basis # qz+t(H)p+p'
O 4
n=2 0 4 E 50.0 8.0
   10.0 5.0 3.5 2.0
n=2 1 4 E 10.0 8.0
   10.0 5.0 3.5 2.0
n=3 2 2 E 40.0 9.0 Q  6.0 0.00
   10.0 2.2
n=4 3 1 E 50.0 9.0 Q 17.0 0.40
   10.0
H 3
n=1 0 4 E 50.0 9.0
   10.0 5.0 3.5 2.0
n=2 1 3 E 50.0 9.0 Q  3.5 0.00
   10.0 2.0 4.0
n=3 2 1 E 50.0 9.0 Q 16.0 0.80
   10.0
%endblock PAO.Basis
```

```
%block PAO.Basis # qz+t(H)p+d(H)p'
O 4
n=2 0 4 E 50.0 8.0
   10.0 5.0 3.5 2.0
n=2 1 4 E 10.0 8.0
   10.0 5.0 3.5 2.0
n=3 2 2 E 40.0 9.0 Q  6.0 0.00
   10.0 2.2
n=4 3 1 E 50.0 9.0 Q 17.0 0.40
   10.0
H 3
n=1 0 4 E 50.0 9.0
   10.0 5.0 3.5 2.0
n=2 1 3 E 50.0 9.0 Q  3.5 0.00
   10.0 2.0 4.0
n=3 2 2 E 50.0 9.0 Q 16.0 0.80
   10.0 2.0
%endblock PAO.Basis

%block PAO.Basis # qz+tp+d(H)p'
O 4
n=2 0 4 E 50.0 8.0
   10.0 5.0 3.5 2.0
n=2 1 4 E 10.0 8.0
   10.0 5.0 3.5 2.0
n=3 2 3 E 40.0 9.0 Q  6.0 0.00
   10.0 2.0 3.0
n=4 3 1 E 50.0 9.0 Q 17.0 0.40
   10.0
H 3
n=1 0 4 E 50.0 9.0
   10.0 5.0 3.5 2.0
n=2 1 3 E 50.0 9.0 Q  3.5 0.00
   10.0 2.0 4.0
n=3 2 2 E 50.0 9.0 Q 16.0 0.80
   10.0 2.0
%endblock PAO.Basis

%block PAO.Basis # qz+tp+dp'
O 4
n=2 0 4 E 50.0 8.0
   10.0 5.0 3.5 2.0
n=2 1 4 E 10.0 8.0
   10.0 5.0 3.5 2.0
n=3 2 3 E 40.0 9.0 Q  6.0 0.00
   10.0 2.0 3.0
n=4 3 2 E 50.0 9.0 Q 17.0 0.40
   10.0 1.7
H 3
n=1 0 4 E 50.0 9.0
   10.0 5.0 3.5 2.0
n=2 1 3 E 50.0 9.0 Q  3.5 0.00
   10.0 2.0 4.0
n=3 2 2 E 50.0 9.0 Q 16.0 0.80
   10.0 2.0
%endblock PAO.Basis
```
